# Supplementary material for: FootstepNet: an Efficient Actor-Critic Method for Fast On-line Bipedal Footstep Planning and Forecasting
Source: arXiv:2403.12589 source file (2024-12-17)
Supplement: Supplementary file 1 [file appendix.tex]

%\section*{APPENDIX}

%Appendixes should appear before the acknowledgment.
%\vspace{-0.2cm} 

\section*{ACKNOWLEDGMENT}
Acknowledgment goes here.
